# Supplementary material for: Quantiled conditional variance, skewness, and kurtosis by Cornish-Fisher expansion
Source: arXiv:2302.06799 ancillary file (2023-06-06)
Supplement: Supplementary file 1 [file Supplementary_materials.pdf]

# SUPPLEMENTARY MATERIALS TO “QUANTILED CONDITIONAL VARIANCE, SKEWNESS, AND KURTOSIS BY CORNISH-FISHER EXPANSION”

## Appendix: Proofs.

*Proof of Theorem 3.1.* By noting that

$$(A.1) \quad \widehat{\boldsymbol{\theta}}_t - \boldsymbol{\theta}_t = \mathbf{M}_n^{-1} \left( \frac{\mathbf{Z}' \boldsymbol{\varepsilon}_t}{n} \right),$$

the results follow from Assumptions 3.1–3.2 and the continuous mapping theorem.  $\square$

*Proof of Theorem 3.2.* By (A.1), Assumption 3.3, and Corollary 4.24 in [White \(2001\)](#),

$$(A.2) \quad (\mathbf{M}_n^{-1} \mathbf{V}_{t,n} \mathbf{M}_n^{-1})^{-1/2} \sqrt{n}(\widehat{\boldsymbol{\theta}}_t - \boldsymbol{\theta}_t) = (\mathbf{M}_n^{-1} \mathbf{V}_{t,n} \mathbf{M}_n^{-1})^{-1/2} \mathbf{M}_n^{-1} \left( \frac{\mathbf{Z}' \boldsymbol{\varepsilon}_t}{\sqrt{n}} \right) \\ \xrightarrow{d} N(0, \mathbf{I}) \text{ as } n \rightarrow \infty.$$

Define a three-dimensional function  $\mathbf{g}(\mathbf{x}) = (g_1(\mathbf{x}), g_2(\mathbf{x}), g_3(\mathbf{x}))$  for  $\mathbf{x} = (x_1, x_2, x_3, x_4)$ , where  $g_1(\mathbf{x}) = x_2^2$ ,  $g_2(\mathbf{x}) = 6x_3/x_2$ , and  $g_3(\mathbf{x}) = 24x_4/x_2 + 3$ . By Taylor’s expansion and the fact that  $\widehat{\boldsymbol{\theta}}_t - \boldsymbol{\theta}_t = O_p(n^{-1/2})$  from (A.2), we have

$$g_i(\widehat{\boldsymbol{\theta}}_t) = g_i(\boldsymbol{\theta}_t) + [\nabla_{\mathbf{x}} g_i(\boldsymbol{\theta}_t)]'(\widehat{\boldsymbol{\theta}}_t - \boldsymbol{\theta}_t) + O_p\left(\frac{1}{n}\right)$$

for  $i = 1, 2, 3$ , where  $\nabla_{\mathbf{x}}$  is the gradient operator. Consequently, since  $h_t = g_1(\boldsymbol{\theta}_t)$ ,  $s_t = g_2(\boldsymbol{\theta}_t)$ ,  $k_t = g_3(\boldsymbol{\theta}_t)$ ,  $\widehat{h}_t = g_1(\widehat{\boldsymbol{\theta}}_t)$ ,  $\widehat{s}_t = g_2(\widehat{\boldsymbol{\theta}}_t)$ , and  $\widehat{k}_t = g_3(\widehat{\boldsymbol{\theta}}_t)$ , it follows that

$$(A.3) \quad \sqrt{n} \begin{pmatrix} \widehat{h}_t - h_t \\ \widehat{s}_t - s_t \\ \widehat{k}_t - k_t \end{pmatrix} = \mathbf{R}_t \sqrt{n}(\widehat{\boldsymbol{\theta}}_t - \boldsymbol{\theta}_t) + O_p\left(\frac{1}{\sqrt{n}}\right),$$

where

$$\mathbf{R}_t = \begin{pmatrix} 0 & 2\beta_{1t} & 0 & 0 \\ 0 & -6\beta_{2t}/\beta_{1t}^2 & 6/\beta_{2t} & 0 \\ 0 & -24\beta_{3t}/\beta_{1t}^2 & 0 & 24/\beta_{2t} \end{pmatrix}.$$

By (A.2)–(A.3), we know that  $\hat{h}_t$ ,  $\hat{s}_t$ , and  $\hat{k}_t$  are  $\sqrt{n}$ -consistent, but they are not asymptotically normal since  $\mathbf{R}_t$  is a random rather than deterministic matrix.  $\square$

**Additional simulations on the selection of  $p^*$ .** In Procedure 4.1, we use the CAViaR method to obtain the ECQs  $\{\hat{Q}_t(\alpha_i)\}_{t=1}^T$ , and then discard some of  $\{\hat{Q}_t(\alpha_i)\}_{t=1}^T$  with p-values of DQ test less than  $p^* = 0.1$ . Below, we examine the performance of QCM method with respect to the choice of  $p^*$ .

Under the same simulation settings as before and the results of 100 replications, we plot the boxplots of  $\Delta_{h,t}$ ,  $\Delta_{s,t}$ , and  $\Delta_{k,t}$  for  $t = 1, \dots, 10$  in Figs B1–B3 across four different choices of  $p^*$  (that is,  $p^* = 0, 0.1, 0.3$ , and  $0.5$ ), where  $\hat{Q}_t(\alpha_i)$  is mis-specified computed from the CAViaR method. From these three figures, we find that the performance of QCMs is robust to the choice of  $p^*$ , except that a larger  $p^*$  tends to deliver more outliers of  $\Delta_{s,t}$  and  $\Delta_{k,t}$ . This exception is probably because a large value of  $p^*$  makes the value of  $n_0$  become small and thus reduce the efficiency of the OLS estimator  $\hat{\theta}_t$  and the QCMs.

Since the graphic difference of QCMs with respect to the choice of  $p^*$  in Figs B1–B3 is subtle, we further plot the mean values and standard deviations of  $\Delta_{h,t}$ ,  $\Delta_{s,t}$ , and  $\Delta_{k,t}$  for  $t = 1, \dots, 10$  under four different values of  $p^*$  in Figs B4 and B5, respectively, based on the results of 100 replications. From Figs B4–B5, we find that although the estimation errors of QCMs generally have the smallest deviation when  $p^* = 0$ , they do not always have the smallest mean value under this choice of  $p^*$ . Therefore, to balance the mean and variance of QCM estimation errors, the choice of  $p^* = 0.1$  seems desirable.

## References.

White, H. (2001). *Asymptotic Theory for Econometricians, Revised edition*. San Diego: Academic Press.

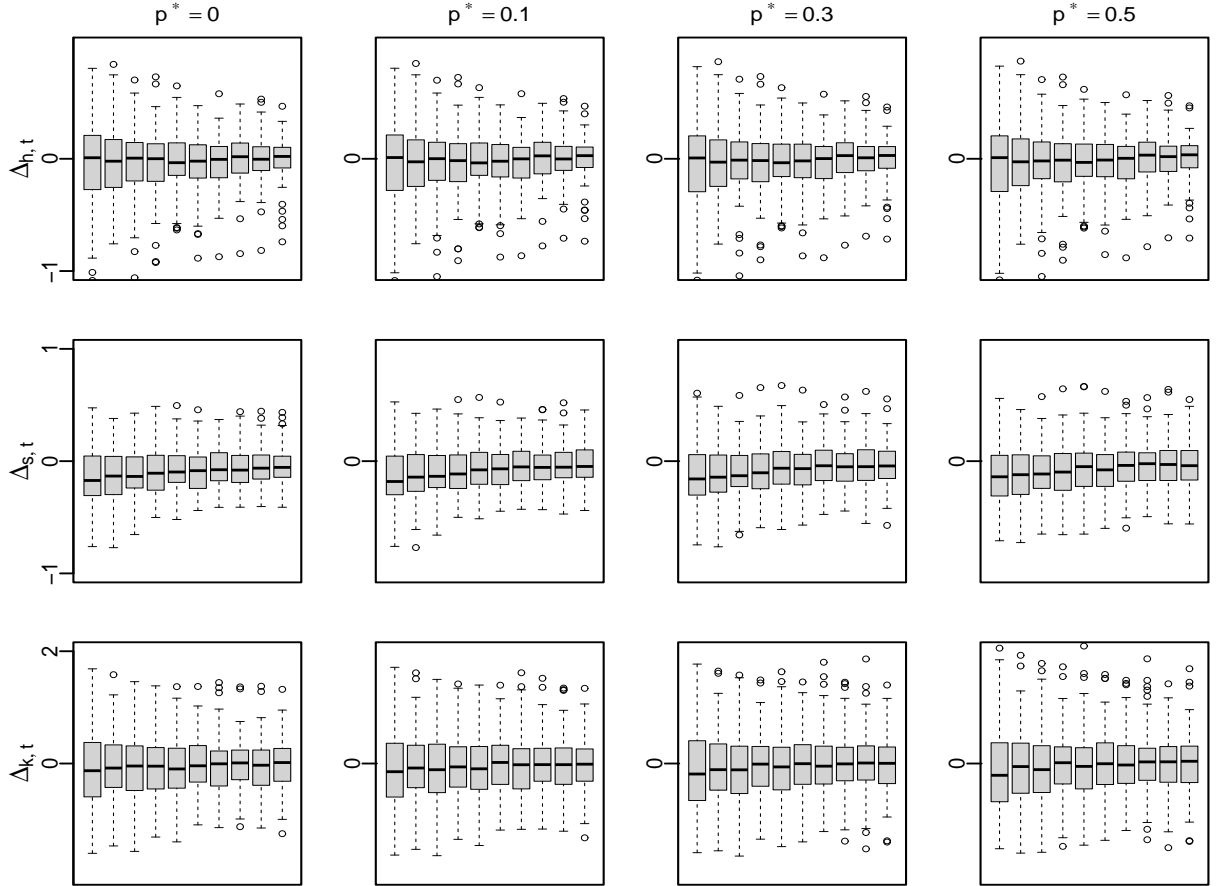

Fig B1: The boxplots of  $\Delta_{h,t}$ ,  $\Delta_{s,t}$ , and  $\Delta_{k,t}$  for  $t = 1, \dots, 10$  under four different choices of  $p^*$ , where the data are generated from the standard GARCH model in (5.1) with  $\eta_t \sim N(0, 1)$ , and  $\hat{Q}_t(\alpha_i)$  are estimated via the CAViaR method.

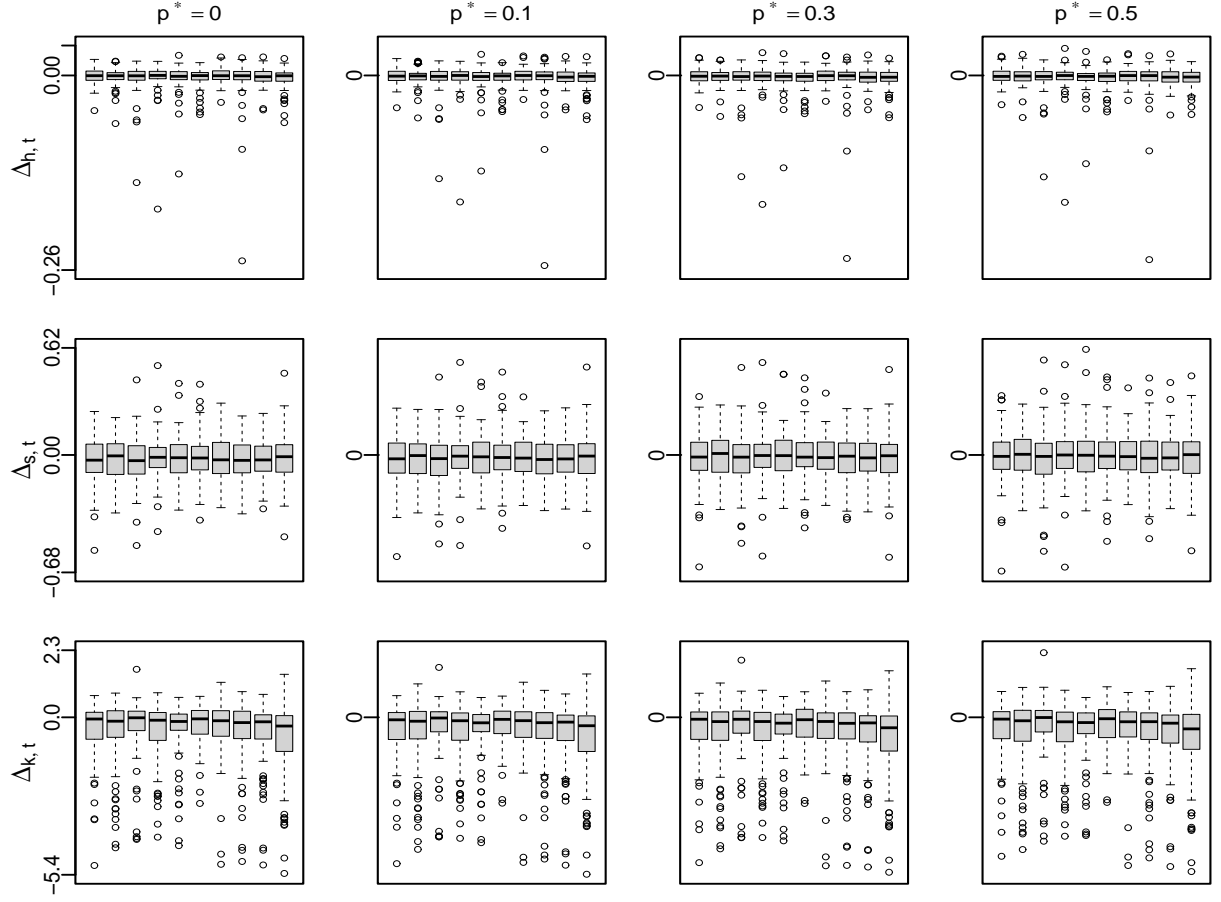

Fig B2: The boxplots of  $\Delta_{h,t}$ ,  $\Delta_{s,t}$ , and  $\Delta_{k,t}$  for  $t = 1, \dots, 10$  under four different choices of  $p^*$ , where the data are generated from the standard GARCH model in (5.1) with  $\eta_t \sim ST_{\nu_t}$ , and  $\hat{Q}_t(\alpha_i)$  are estimated via the CAViaR method.

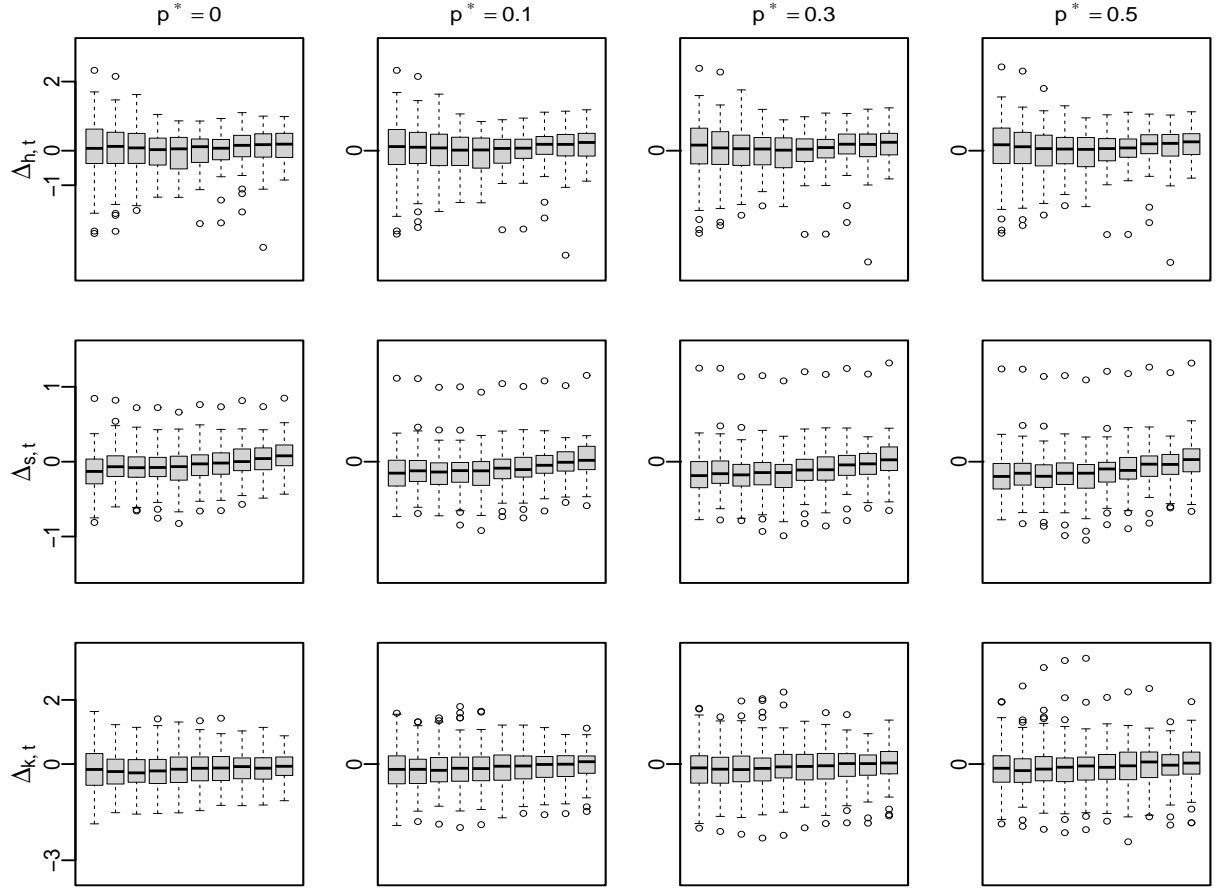

Fig B3: The boxplots of  $\Delta_{h,t}$ ,  $\Delta_{s,t}$ , and  $\Delta_{k,t}$  for  $t = 1, \dots, 10$  under four different choices of  $p^*$ , where the data are generated from the ARMA-MN-GARCH model in (5.4), and  $\hat{Q}_t(\alpha_i)$  are estimated via the CAViaR method.

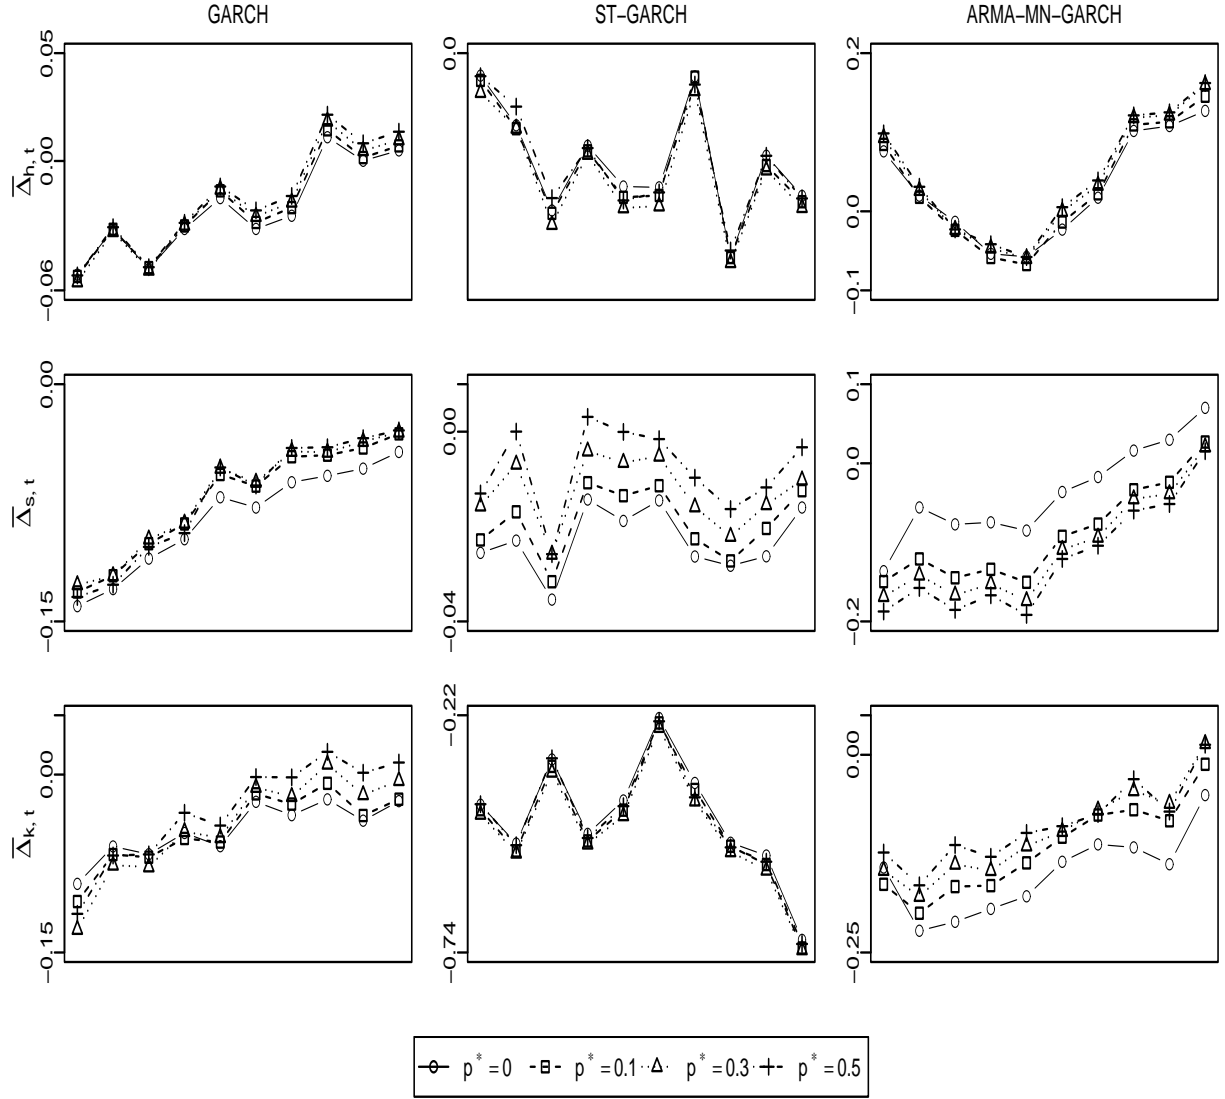

Fig B4: The mean values of  $\Delta_{h,t}$ ,  $\Delta_{s,t}$ , and  $\Delta_{k,t}$  (denoted by  $\bar{\Delta}_{h,t}$ ,  $\bar{\Delta}_{s,t}$ , and  $\bar{\Delta}_{k,t}$ , respectively) for  $t = 1, \dots, 10$  under four different choices of  $p^*$ , where  $\hat{Q}_t(\alpha_i)$  are estimated via the CAViaR method.

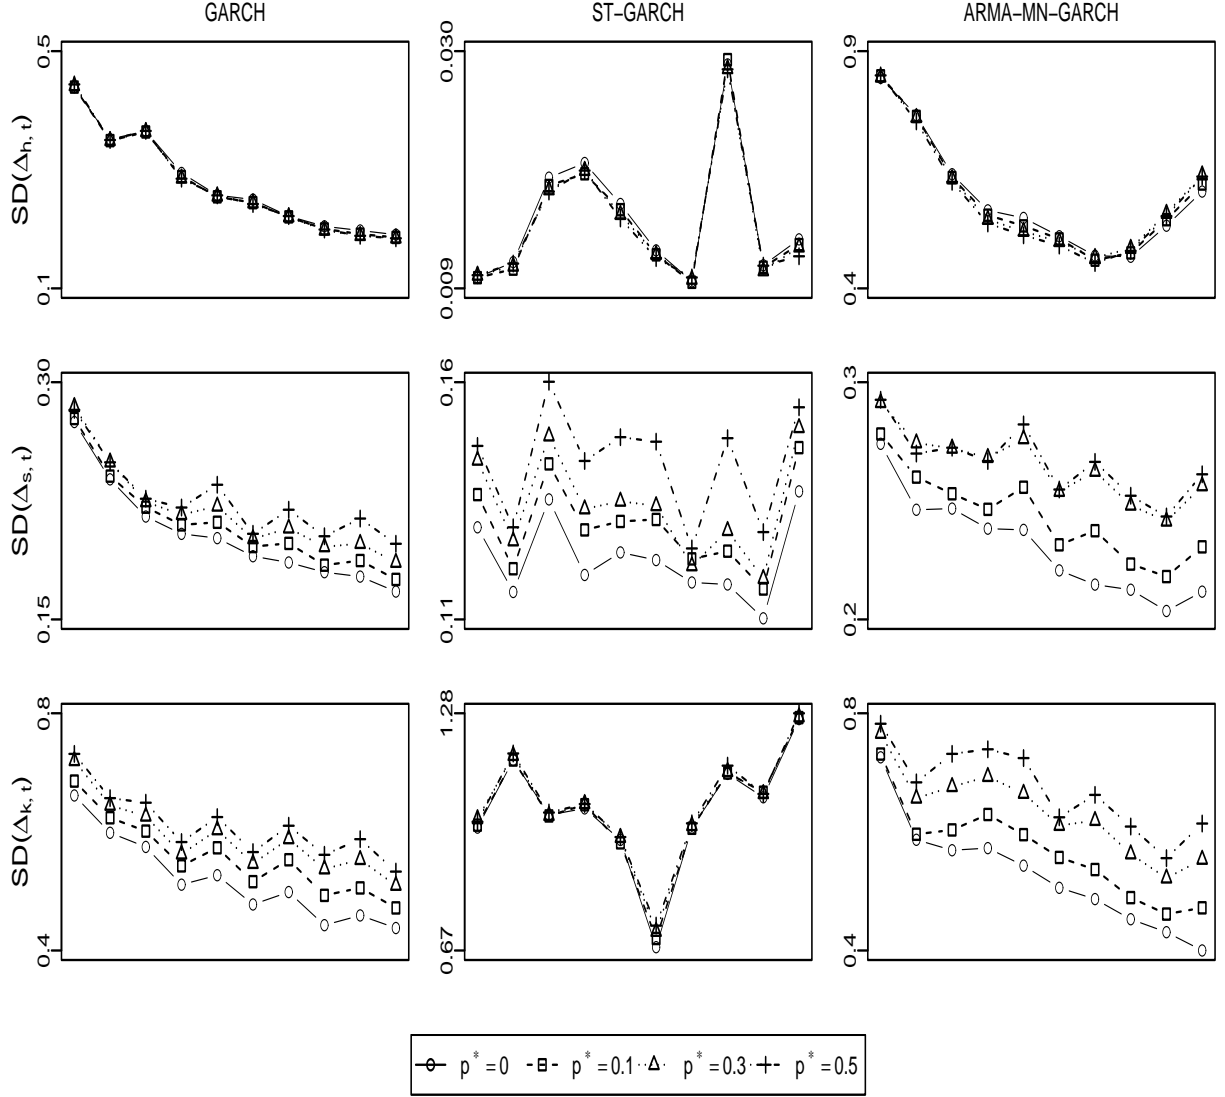

Fig B5: The standard deviations of  $\Delta_{h,t}$ ,  $\Delta_{s,t}$ , and  $\Delta_{k,t}$  (denoted by  $SD(\Delta_{h,t})$ ,  $SD(\Delta_{s,t})$ , and  $SD(\Delta_{k,t})$ , respectively) for  $t = 1, \dots, 10$  under four different choices of  $p^*$ , where  $\hat{Q}_t(\alpha_i)$  are estimated via the CAViaR method.
